# Supplementary material for: Writing on the Facade of RWTH ICT Cubes: Cost Constrained Geometric Huffman Coding
Source: arXiv:1106.5675 source file (2011-06-28)
Supplement: Supplementary file 1 [file appendix.tex]

\section{Proof of Proposition~\ref{prop:geometry}}
